# Supplementary material for: Chemical Raman Enhancement of Organic Adsorbates on Metal Surfaces
Source: arXiv:1011.1873 ancillary file (2010-11-08)
Supplement: Supplementary file 1 [file Supplementary_Mat.pdf]

# Supplementary material

## Chemical Raman Enhancement of Organic Adsorbates at Metal Surfaces

A. T. Zayak[1,2], Y. S. Hu[3], H. Choo[1,2], J. Bokor[1,2], S. Cabrini[1], P. J. Schuck[1], and J. B. Neaton[1]

[1] *Molecular Foundry, Lawrence Berkeley National Laboratory, Berkeley, CA 94720, USA*
[2] *Department of Electrical Engineering and Computer Sciences, UC Berkeley, Berkeley, CA 94720-1770, USA*
[3] *Bioengineering Department, Rice University, Houston, TX77005*
*Electronic address: jbneaton@lbl.gov*

### Electronic structure calculations

All first-principles density functional theory[1] calculations are performed using the Vienna Ab-initio Simulations Package (VASP) and within the generalized gradient approximation (GGA) of Perdew, Burke, and Erzenhof (PBE)[2]. Projector-augmented wave potentials[3,4,5,6] are employed to model the electron-ion interaction. The kinetic energy cut-off is set to 400 eV, and 800 eV for the augmentation charges. These values are used throughout all calculations for the sake of consistency, and result in well converged structural and vibrational properties, and binding energies. The equilibrium lattice parameter for gold was obtained by relaxing bulk *fcc* Au with a 12 × 12 × 12 Monkhorst-Pack k-point mesh, resulting in 4.17 Å, within 2.2% of the experimental value of 4.078 Å at room temperature[7].

### Binding geometries

The isolated BT molecule in our calculations has a planar geometry, with the S-H bond lying in the same plane as the phenyl ring, and a C-S-H angle of 96.7 degrees, in agreement with previous calculations[8].

For the adsorbate, four different high-symmetry binding geometries are considered, as shown in Fig. 1a (in the paper): bridge ($E_B$=0.192 eV), *fcc* hollow ($E_B$= 0.219 eV), adatom site ($E_B$=0.446 eV), and hydrogenated adatom ($E_B$=0.795 eV), where the binding energy, $E_B$, is calculated as ($C_6H_5SH$ + Au $\rightarrow$ $C_6H_5S$@Au +0.5$H_2$)[9]. Calculated binding energies are in agreement with an unpublished calculation[10].

The first three geometries differ in the number of gold atoms bound to sulfur. The adatom geometry, with a single S-Au bond of length 2.3 Å, binds most strongly, with a Au-S-C dihedral angle of 112 degrees. The bridge site has an S atom bound to two Au atoms, with the phenyl ring oriented at about 60 degrees relative to the normal of the surface, with an S-Au bond length 2.48 Å. The *fcc* hollow site involves the binding of sulfur to three gold atoms, with ring oriented vertically relative to the Au surface, with S-Au bond length 2.46 Å. Both our *fcc* hollow and bridge geometries agree well with previous DFT studies[11].

The hydrogenated adatom geometry appears to be the most stable, however if we consider estimated desorption barriers, we obtain: bridge ($E_B$=1.57 eV), *fcc* hollow ($E_B$= 1.60 eV), adatom site ($E_B$=1.81 eV), and hydrogenated adatom ($E_B$=0.80 eV), and the latter appears to be the least stable. The first three numbers are computed with a reference to the gas-phase molecule without H, and provide an estimate of the desorption barrier assuming that the H would reattach only after desorption. It was shown experimentally that at low temperatures hydrogen can stay at sulfur, but that at room temperature,

dissociation of the S-H bond usually occurs[12]. Experiments also report that the Raman active S-H stretch mode at 2600 $cm^{-1}$ is not observed in SERS measurements[13]. This suggests that the hydrogenated adatom geometry is less relevant to room-temperature experimental data. It is, however, very useful for our theoretical analysis, because we show that is has negligible chemical enhancement. We use this property to isolate the interfacial contribution to chemical enhancement in the other geometries.

## Vibrational modes

Vibrational frequencies and corresponding phonon eigenvectors are obtained by diagonalization of a truncated dynamical matrix treating only BT atoms, and Au atoms directly bonded with sulfur. The remainder of the Au atoms in our slab are treated in an infinite mass approximation. Incorporation of additional Au atoms from the substrate into our dynamical matrices did not alter mode frequencies or eigenvalues. A similar approach is taken in Ref.[14] for studying vibrations of CO molecules on Pt(111) surface, where it was demonstrated that including additional metal atoms in the dynamical matrix does not have considerable effect on the vibrations of the molecule. The dynamical matrix of the system is constructed by finite differences, i.e. displacing each atom from their equilibrium positions along each Cartesian direction by 0.03 Å, large enough to obtain a good forces-to-noise ratio while still in the harmonic regime. We used Hellmann-Feynman forces induced on all atoms of the system to construct a symmetrized form of the dynamical matrix, as follows[15]:

$$D_{ij}^{\alpha\beta} = -\frac{1}{2}\left[\frac{F_i^\alpha\left(\{\mathbf{r}\}+d_j^\beta\right)-F_i^\alpha\left(\{\mathbf{r}\}-d_j^\beta\right)}{2d_j^\beta}+\frac{F_j^\beta\left(\{\mathbf{r}\}+d_i^\alpha\right)-F_j^\beta\left(\{\mathbf{r}\}-d_i^\alpha\right)}{2d_i^\alpha}\right] \qquad \text{(S1)}$$

In the above, $F_j^\alpha$ is the force on atom $\alpha$ in the direction $j$ and $\{\mathbf{r}\}\pm d_i^\beta$ is the atomic configuration where only the atom $\beta$ is displaced along direction $i$ from its equilibrium position. Diagonalization of the dynamical matrix leads to frequencies $\omega_n$ and corresponding normalized mass-weighted eigenmodes for atomic displacements $\tilde{Q}_n$. The actual displacements are given by $Q_{\alpha,j}^n = \tilde{Q}_{\alpha,j}^n / \sqrt{M_\alpha}$ .

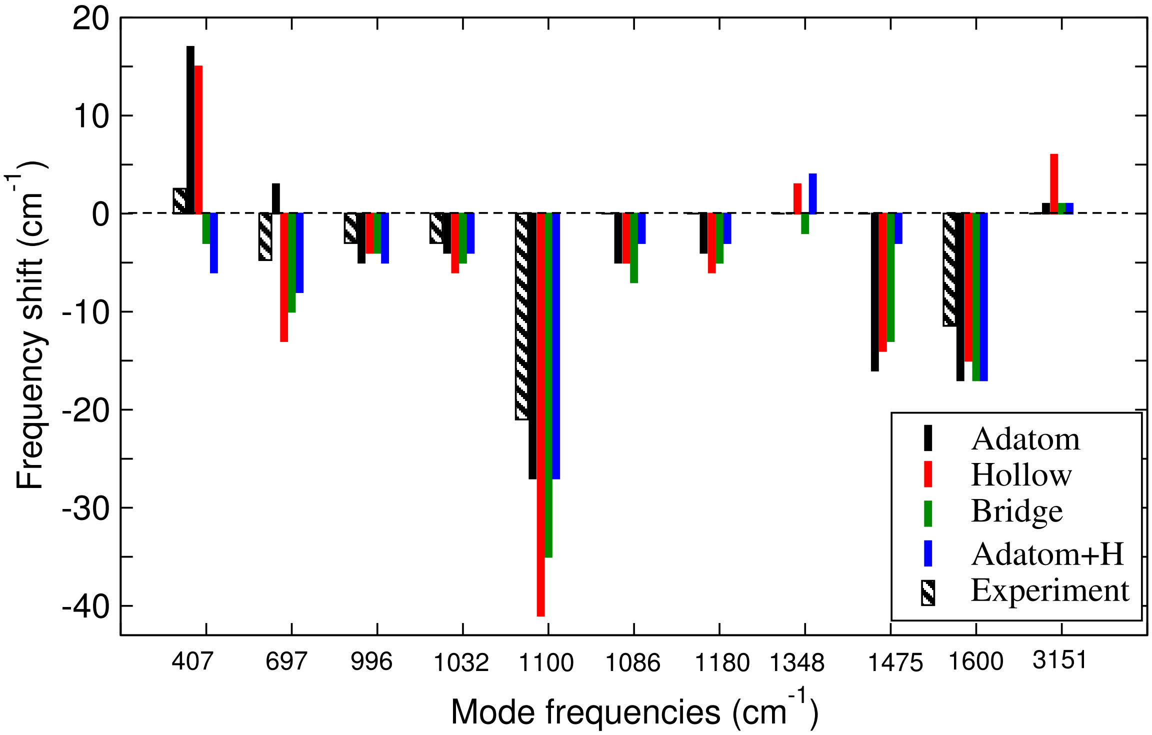


FIGURE S1. Frequency shift for selected vibrational modes of BT, calculated as $\omega_{(\text{Adsorbed BT})} - \omega_{(\text{Isolated BT})}$ . Positive value means that frequency shifts up at adsorption. Agreement with experimental data is clearly seen.

Upon adsorption, frequencies of vibrational modes change as summarized in Fig. S1. It is surprisingly noticeable that modes, which exhibit stronger frequency shifts, also demonstrate stronger chemical enhancement. In most cases CE correlates with a downshift of the frequency. Exception is the 407 $cm^{-1}$ mode which is related to the motion of sulfur atom, being more sensitive to changes in the bonding environment as compared to other modes.

## Raman Tensor and Intensities

In this work, for the isolated BT (gas phase) we compute the full Raman tensor and use the standard procedure for averaging, which approximates cross section of a molecule in a completely orientationally-disordered solution or gas-phase.

For BT adsorbates on Au surfaces, we calculate only one component of the Raman tensor, $R^n_{zz}$, where n is a mode index, and z is the Cartesian direction normal to the substrate surface. In this work, we define this quantity as follows:

$$R^n_{ij} = \frac{d\alpha_{ij}}{dQ_n} \approx \frac{\alpha_{ij}\left(\{\mathbf{r}\}+Q_n\right)-\alpha_{ij}\left(\{\mathbf{r}\}-Q_n\right)}{2Q_n}, \qquad \text{(S2)}$$

where is the static polarizability tensor, $\{\mathbf{r}\} \pm Q_n$ are atomic coordinates distorted by the n-th vibrational mode. The static polarizability tensor $\alpha_{ij}$ is a second derivative with respect to electric field,

$$\alpha_{ij} = \frac{\partial^2 E_{DFT}}{\partial\varepsilon_i \partial\varepsilon_j} \qquad \text{(S3)}$$

approximated with a second-order finite-difference expression[16], i.e.

$$\frac{\partial^2 E}{\partial \varepsilon_x^2} \approx \frac{E_{i+2,j} - 2E_{i+1,j} + E_{i,j}}{\Delta \varepsilon_x^2}$$

$$\frac{\partial^2 E}{\partial \varepsilon_x \partial \varepsilon_y} \approx \frac{E_{i+1,j+1} - E_{i+1,j} - E_{i,j+1} + E_{i,j}}{\Delta \varepsilon_x \Delta \varepsilon_y}, \tag{S4}$$

where $E$ is the total energy and $\varepsilon_x$ is the *x*-component of the electric field.

The electric field is applied via a saw tooth potential[17]. For our supercell, we use a gradient of 1 mV/Å. The standard expression is used for calculating the differential Raman cross section[18]:

$$\left(\frac{d\sigma}{d\Omega}\right)_n = \frac{2\pi^2 h\left(\omega_{Laser} - \omega_n\right)^4}{c\omega_n} \left|\vec{\varepsilon}_i \cdot \hat{R} \cdot \vec{\varepsilon}_s\right|^2 \frac{1}{1 - \exp\left(-\frac{hc\omega_n}{kT}\right)} \tag{S5}$$

In the case of solution or gas phase cross section, $\left|\vec{\varepsilon}_i \cdot \hat{R} \cdot \vec{\varepsilon}_s\right|$ is approximated by a rotationally averaged value $I_n^{Raman}$, which takes the form[19,20]

$$I_n^{Raman} = \left(A_n\right)^2 + \frac{7}{45}\left(B_n\right)^2,$$

$$A_n = \frac{1}{3}\sum_j R_{jj}^n ; \quad \left(B_n\right)^2 = \frac{1}{2}\sum_{ij}\left(3R_{ij}^n R_{ij}^n - R_{jj}^n R_{ii}^n\right) \tag{S6}$$

For the adsorbate geometries, we compute only one component of the Raman tensor, $R_{zz}^n$.

In this case we have $I_n^{Raman} = \left(R_{zz}^n\right)^2$.

After substituting numerical values in eq.(S5), Raman cross sections for BT on Au are obtained with the text-book expression[18]:

$$\left(\frac{d\sigma}{d\Omega}\right)_n \left[\frac{cm^2}{sr}\right] = 5.8\cdot 10^{-46} \frac{\left[\left(10^7 / \lambda_{Laser}[nm]\right) - \omega_n[cm^{-1}]\right]}{\omega_n[cm^{-1}]} I_n^{Raman}\left[Å/amu\right] \cdot \left(1-\exp\left(-\frac{\omega_n[cm^{-1}]}{201.56}\right)\right)^{-1} \quad \text{(S7)}$$

We verified our approach by comparing the Raman spectrum of gas-phase benzene thiol with experiments[21,22] and previous calculations[23]. The overall agreement is good, although the relative intensities of our gas phase calculation show some discrepancies with experiment, the most prominent of which is our underestimated intensity for the 996 $cm^{-1}$ mode. We tested various calculation schemes within the same DFT framework (different pseudopotentials, different codes, e.g. PWSCF, etc) and obtained results consistent with our plane wave PBE picture. Similar underestimated 996 $cm^{-1}$ mode was reported recently in Ref.[24]. Calculations done with B3LYP/6-311+G** improve on this disagreement[23]. However, we observe the same trends for the 996 $cm^{-1}$ mode for the adsorbate geometries as well. We, thus, conclude that as long as we are consistent with the basis set we use, our analysis of the chemical enhancement should be correct.

Results for calculated adsorbate Raman cross sections are given in Table S1. We note that in the table, the gas phase cross sections are not averaged, but calculated from $I_n^{Raman} = \left(R_{zz}^n\right)^2$ only, with the molecule positioned in exactly the same orientation with respect to the z axis, as the corresponding geometry of the adsorbate.

TABLE S1

Calculated vibrational frequencies and Raman cross sections. Corresponding isolated molecule data is given in brackets. Adatom and adatom+H use the same isolated molecule reference.

| Adatom | | Hollow | | Bridge | | Adatom+H | |
|---|---|---|---|---|---|---|---|
| ν [$cm^{-1}$] | $R_{zz}$ [$10^{-31}$ $cm^2$/sr] | ν [$cm^{-1}$] | $R_{zz}$ [$10^{-31}$ $cm^2$/sr] | ν [$cm^{-1}$] | $R_{zz}$ [$10^{-31}$ $cm^2$/sr] | ν [$cm^{-1}$] | $R_{zz}$ [$10^{-31}$ $cm^2$/sr] |
| (407)<br>424 | (0.21)<br>68.74 | (407)<br>422 | (1.51)<br>5.81 | (407)<br>404 | (0.15)<br>3.18 | (407)<br>401 | (0.21)<br>0.65 |
| (697)<br>700 | (0.05)<br>7.10 | (697)<br>684 | (0.006)<br>3.62 | (697)<br>687 | (0.03)<br>0.66 | (697)<br>689 | (0.05)<br>0.44 |
| (996)<br>991 | (0.56)<br>23.73 | (996)<br>992 | (0.93)<br>2.10 | (996)<br>992 | (0.20)<br>1.43 | (996)<br>995 | (0.56)<br>2.61 |
| (1032)<br>1028 | (0.60)<br>58.14 | (1032)<br>1026 | (0.71)<br>15.28 | (1032)<br>1027 | (0.20)<br>5.60 | (1032)<br>1028 | (0.60)<br>4.52 |
| (1100)<br>1073 | (0.46)<br>150.28 | (1100)<br>1059 | (0.72)<br>20.73 | (1100)<br>1065 | (0.07)<br>7.91 | (1100)<br>1079 | (0.46)<br>5.93 |
| (1086)<br>1081 | (0.08)<br>22.92 | (1086)<br>1081 | (0.035)<br>0.51 | (1086)<br>1079 | (0.005)<br>0.01 | (1086)<br>1083 | (0.08)<br>0.21 |
| (1180)<br>1176 | (0.11)<br>9.16 | (1180)<br>1174 | (0.07)<br>0.39 | (1180)<br>1175 | (0.0004)<br>0.18 | (1180)<br>1177 | (0.11)<br>0.62 |
| (1348)<br>1348 | (0.052)<br>2.37 | (1348)<br>1351 | (0.004)<br>0.02 | (1350)<br>1346 | (0.001)<br>0.01 | (1348)<br>1352 | (0.052)<br>0.28 |
| (1475)<br>1459 | (0.001)<br>21.50 | (1475)<br>1461 | (0.0005)<br>1.56 | (1475)<br>1462 | (0.005)<br>0.7 | (1475)<br>1472 | (0.001)<br>0.41 |
| (1600)<br>1583 | (0.19)<br>136.69 | (1600)<br>1585 | (1.03)<br>16.58 | (1599)<br>1583 | (0.076)<br>4.73 | (1600)<br>1590 | (0.19)<br>2.27 |
| (3151)<br>3152 | (0.91)<br>5.26 | (3151)<br>3157 | (1.128)<br>5.63 | (3151)<br>3152 | (0.16)<br>0.74 | (3151)<br>3152 | (0.91)<br>4.52 |

## Geometric correlation

Intuitively, because the BT HOMO is a $\pi$ orbital, BT vibrational modes that break chemical conjugation of the carbon ring might be expected to have the largest deformation potential, $\partial\omega_H/\partial Q_n$ . An approximate way of quantifying this picture is to use a correlation function

$$\Omega = \sum_i \left(d_i^{(C-C)} - \bar{d}^{(C-C)}\right)^2 + \left(\Delta d^{(S-Au)}\right)^2, \qquad \bar{d}^{(C-C)} = \frac{1}{6}\sum_i d_i^{(C-C)} \tag{S8}$$

This correlation function describes the deviation of C-C bonds from their mean value, with an additional contribution from the stretching of the S-Au bond. For modes in which deviation of such bonds are the same, the π-system is approximately preserved, and $\Omega = 0$; if some bonds become longer than others, $\Omega$ increases. In Fig.S2, we show rough correlation between $\Omega$ and the deformation potential $\partial\omega_H/\partial Q_n$ , indicating that modes that disrupt the $\pi$ system have the largest in chemical enchancements.

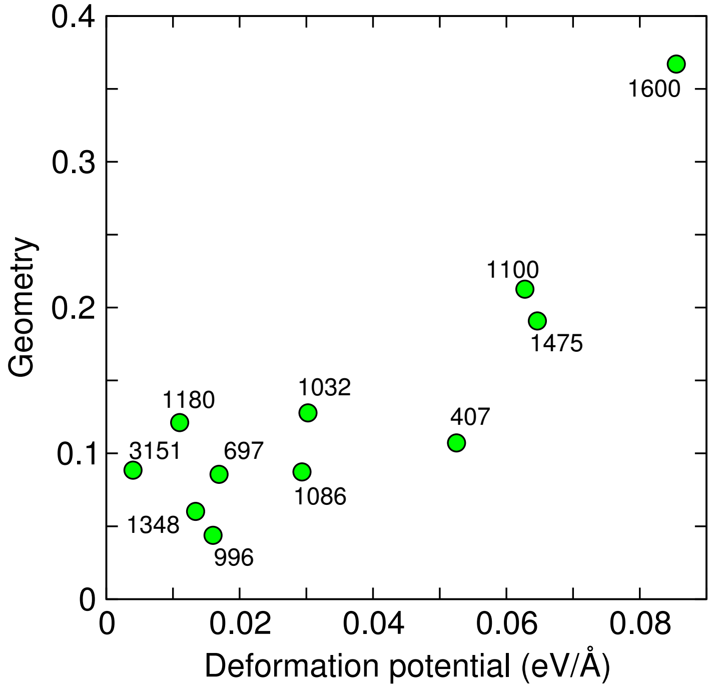

FIGURE S2. An approximate correlation between geometric factors determining breaking of the resonant $\pi$ orbital and the induced deformation potential $\partial\omega_H/\partial Q_n$ .

## Experimental measurements for Raman and SERS

SERS substrates, consisting of roughened SiGe surfaces (Fig. 4a in the paper) coated with 30 nm of Au, were incubated in 3mM benzene thiol solution (Sigma Aldrich W361607) in methanol overnight, then gently rinsed with methanol and dried by nitrogen gas. Raman (neat solution) and SERS spectra were collected at two wavelengths, 632.8 nm and 785 nm, using an inverted microscope set-up coupled to a spectrometer (Acton SpectraPro 2300i) equipped with a liquid-nitrogen-cooled charge-coupled device (CCD) camera. Examples of our measurements are shown in Fig.S3.

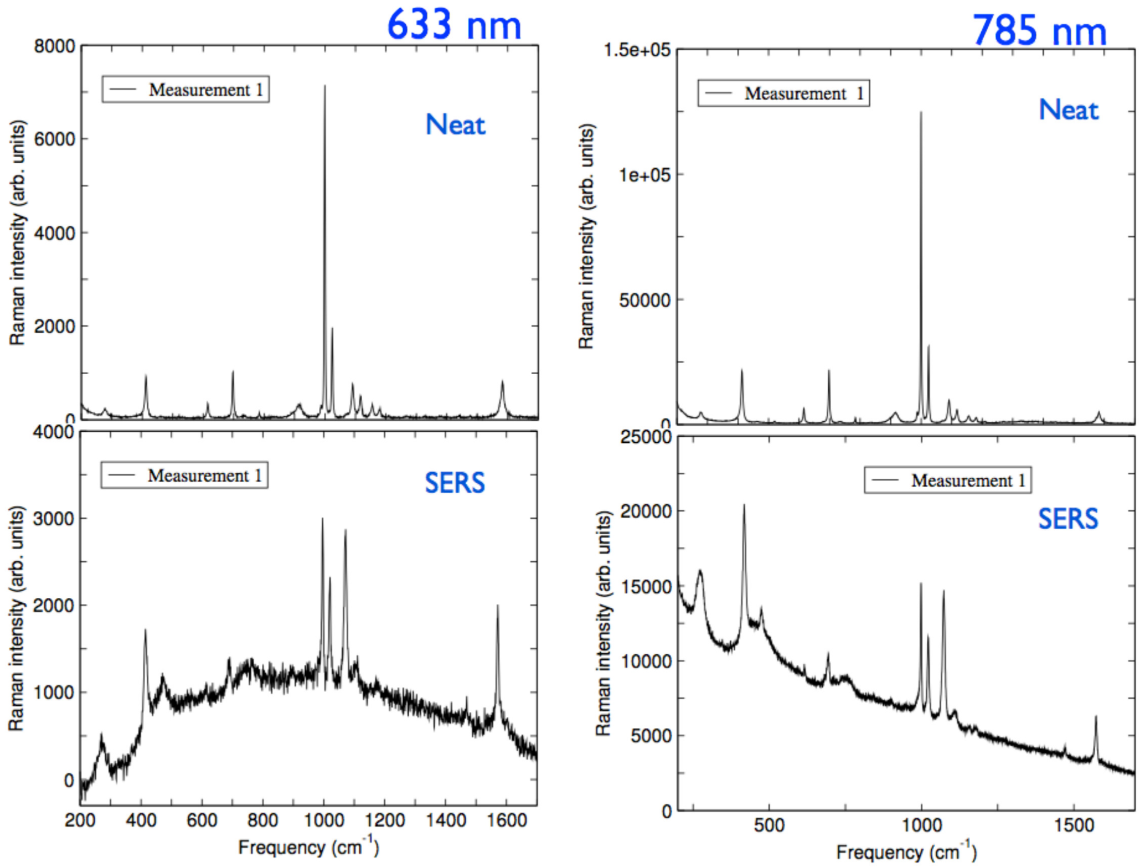

FIGURE S3. Raman and SERS spectra taken at two different wavelengths, 633 nm and 785 nm.

Comparison of two Raman measurements from neat BT shows that our conventional (neat) Raman spectra are probe frequency dependent. One can see differences by comparing intensities of peaks at 407cm$^{-1}$ and 1600 cm$^{-1}$. In measurements taken with 785 nm wavelength, Raman intensities degrade at higher vibrational frequencies. Surprisingly, the same intensity degradation is seen in SERS spectra (see Fig. S3). There is a possibility of an artifact associated with our particular measurements set up. However, similar trends have been observed in experimental data reported by other groups. In order to overcome this problem when taking ratios between Raman and SERS data, we compare only spectra taken at the same laser wavelength. Our analysis shown below demonstrates that this approach works very well.

## Analysis of the experimental data – extracting relative chemical enhancement

To estimate the chemical enhancement and compare with theory, we use the following novel approach for extracting chemical enhancements: After subtracting the fluorescence background, we normalize ratios of neat Raman and SERS spectra peak heights to the 996 cm$^{-1}$ mode, which has only a modest enhancement from our calculations. Assuming the electromagnetic enhancement is the same for all modes, this relative enhancement will reflect only the chemical enhancement. Remarkably, various experiments[21,22] show consistent agreement with our calculations, despite the fact that measurements were done on different substrates, see Fig.S4.

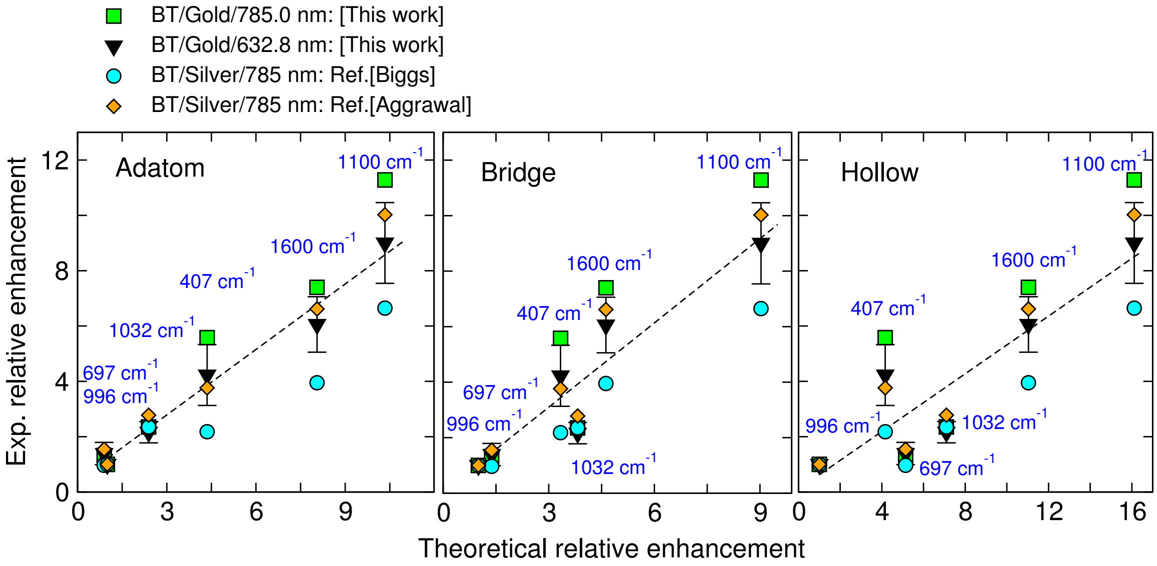


FIGURE S4. Correlations of relative experimental and theoretical chemical enhancements, normalized by the enhancement of the 996 $cm^{-1}$ mode.

**References:**


[1] Kohn W. Nobel Lecture: Electronic structure of matter—wave functions and density functionals. *Rev. Mod. Phys.* **71**, 1253-1266 (1999).

[2] Perdew J. P., Burke K. & Ernzerhof M. Generalized Gradient Approximation Made Simple. *Phys. Rev. Lett.* **77**, 3865-3868 (1996).

[3] Kresse G. & Hafner J. Ab initio molecular dynamics for liquid metals. *Phys. Rev. B* **47**, 558-561 (1993).

[4] Kresse G. & Furthmüller J. Efficient iterative schemes for *ab initio* total-energy calculations using a plane-wave basis set. *Phys. Rev. B* **54**, 11169-11186 (1995).

[5] Kresse G. & D. Joubert D. From ultrasoft pseudopotentials to the projector augmented-wave method. *Phys. Rev. B* **59**, 1758-1775 (1999).

[6] Blöchl P. E. Projector augmented-wave method. *Phys. Rev. B* **50**, 17953-17979 (1994).

[7] Järvi T. T. *et al*. Development of a ReaxFF description for gold. *Eur. Phys. J. B* **66**, 75-79 (2008).

[8] Remacle F. & Kryachko E. S., Thiophenol and thiophenol radical and their complexes with gold clusters $Au_5$ and $Au_6$. *J. Molec. Struct.* **708**, 165-173 (2004).

[9] Letardi S. & Cleri F. Interaction of benzene thiol and thiolate with small gold clusters. *J. Chem. Phys.* **120**, 10062 (2004).

[10] Ning Z., Ji W. & Guo H. Role of contact formation process in transport properties of molecular junctions: conductance of Au/BDT/Au molecular wires. *arXiv:0907.4674v2*.

[11] Bilic A., Reimers J. R. & Hush N. S. The structure, energetics, and nature of the chemical bonding of phenylthiol adsorbed on the Au(111) surface: Implications for density-functional calculations of molecular-electronic conduction. *J. Chem. Phys.* **122**, 094708 (2005).

[12] Maksymovych P. & Yates J. T. Jr. Au Adatomsin Self-Assembly of Benzenethiol on the Au (111) Surface *J. Am. Chem. Soc.* **130**, 7518-7519 (2008)

[13] Cho S. H., Han H. S., Jang D.-J., Kim K. & Kim M. S. Raman Spectroscopic Study of 1,4-Benzenedithiol Adsorbed on Silver. *J. Phys. Chem.* **99**, 10594-10599 (1995)

[14] Lozovoi A. Y. & Alavi A. Vibrational frequencies of CO on Pt(111) in electric field: A periodic DFT study. *J. Electroanal. Chem.* **607**, 140-146 (2007).

[15] Postnikov A. V., Pages O., & Hugel J. Lattice dynamics of the mixed semiconductors (Be,Zn)Se from first-principles calculations. *Phys. Rev. B* **71**, 115206- (2005).

[16] B. D'Acunto, *Computational methods for PDE in mechanics.* Vol. 67 of Series on Advances in Mathematics for Applied Sciences (World Scientific, London, 2004), Chap. Finite differences.

[17] Neugebauer J. & Scheffler M. Adsorbate-substrate and adsorbate-adsorbate interactions of Na and K adlayers on Al(111). *Phys. Rev. B* **46** 16067-16080 (1992)

[18] Le Ru E. C. & Etchegoin P. *Principles of surface-enhanced Raman spectroscopy*. Elsevier, (2009)

[19] M. Cardona in *Light Scattering in Solids II*, Topics in Applied Physics, Vol. 50, Springer-Berlin (1982), p. 24,25

[20] Neugebauer J., Reiher M., Kind C. & Hess B. A. Quantum Chemical Calculation of Vibrational Spectra of Large Molecules—Raman and IR Spectra for Buckminsterfullerene. *J. Comput. Chem.* **23**, 895-910 (2002)

[21] Biggs K. B., Camden J. P., Anker J. N. & Duyne R. P. V. Surface-Enhanced Raman Spectroscopy of Benzenethiol Adsorbed from the Gas Phase onto Silver Film over Nanosphere Surfaces: Determination of the Sticking Probability and Detection Limit Time. *J. Chem. Phys.* **113**, 4581-4586 (2009).

[22] Aggarwal R. L., Farrar L. W., Diebold E. D. & Polla D. L. Measurement of the absolute Raman scattering cross section of the 1584-cm$^{-1}$ band of benzenethiol and the surface-enhanced Raman scattering cross section enhancement factor for femtosecond laser-nanostructured substrates. *J. Raman Spectrosc.* **40**, 1331-1333 (2009).

[23] Li S., Wu D., Xu X. & Gu R. Theoretical and experimental studies on the adsorption behavior of thiophenol on gold nanoparticles. *J. Raman Spectrosc.* **38**, 1436-1443 (2007).

[24] Saikin S. K. *et al*. On the chemical bonding effects in the Raman response: Benzenethiol adsorbed on silver clusters. *Phys. Chem. Chem Phys.* **11**, 9401-9411 (2009).
